# Supplementary material for: Unsupervised Domain Adaptation in the Wild: Dealing with Asymmetric Label Sets
Source: arXiv:1603.08105 source file (2016-03-26)
Supplement: Supplementary file 1 [file supplementary.tex]

\pdfoutput=1
\pagestyle{headings}
\mainmatter
\def\ECCV16SubNumber{925}  % Insert your submission number here
\raggedbottom
\title{Supplementary Material  \\Unsupervised Domain Adaptation in the Wild: Dealing with Asymmetric Label Sets } % Replace with your title

\titlerunning{ECCV-16 submission ID \ECCV16SubNumber}

\authorrunning{ECCV-16 submission ID \ECCV16SubNumber}

\author{Anonymous ECCV submission}
\institute{Paper ID \ECCV16SubNumber}
\maketitle

This document contains supplementary material for our paper.
\section{Plots for Evaluating evolution step of our algorithm}
In section 6.3 of our paper we give an evaluation of the evolving step of our algorithm and give results on Bing as source and Caltech as target. As mentioned in the paper, our measure for analyzing the evolution step is based on the number of target categories present in the final list of selected categories by our algorithm. In figures \ref{fig:e2},\ref{fig:e3},\ref{fig:e4} we give the same result for Bing(source)-Imagenet(target), Caltech(source)-Imagenet(target) and Imagenet(target)-Caltech(source) respectively. The X-axis represents the true number of categories in the target dataset. For each point on the x-axis we average over 10 permutations to get the number of target categories correctly discovered, the number of target categories missed and the number of non-target categories in the final selected set $C_{train}$. Ideally, we expect the selected categories $C_{train}$ to be the label set of the target domain. Hence, we expect a $x=y$ line in the plot. 
% \begin{figure}[H]
%   \centering  
% \subfloat[Using Reprojection Error and  First Local Minima]{\includegraphics[width=0.45\textwidth]{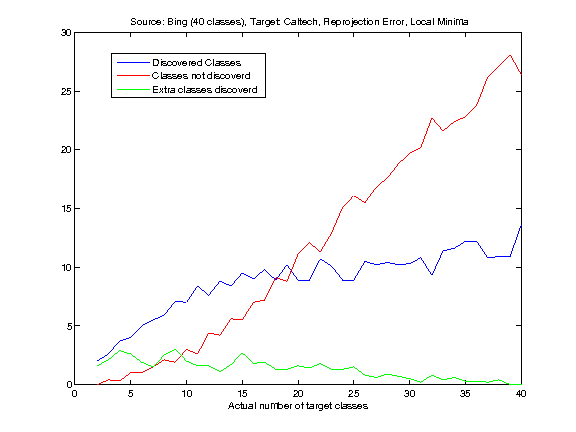}\label{fig:e1f1}} \hfill  
% \subfloat[Using Subspace Alignment Error and First Local Minima]{\includegraphics[width=0.45\textwidth]{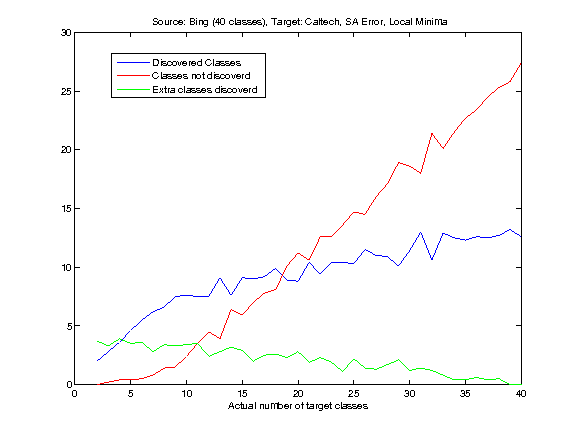}\label{fig:e1f3}}\\
% \subfloat[Using Reprojection Error and Global Minima]{\includegraphics[width=0.45\textwidth]{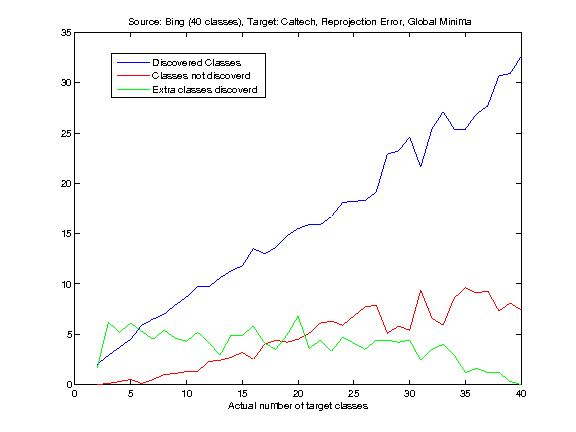}\label{fig:e1f2}}\hfill
% \subfloat[Using Subspace Alignment Error and Global Minima]{\includegraphics[width=0.45\textwidth]{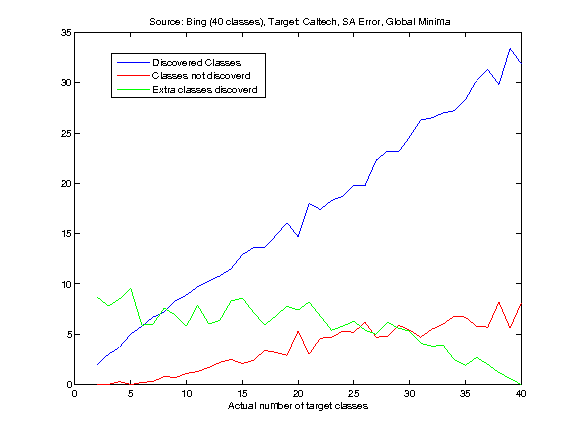}\label{fig:e1f4}}
% \caption{Performance of Evolution Step for different sizes of the target label set (x-axis). Source: Bing, Target: Caltech. Blue: Number of target categories covered in final selected set $C_{train}$. Red: Number of target categories missed in final set. Green: Number of categories not present in target but selected in final set.}\label{fig:e1}
% \end{figure}
\begin{figure}[H]
  \centering
\subfloat[Using Reprojection Error and  First Local Minimum]{\includegraphics[width=0.47\textwidth]{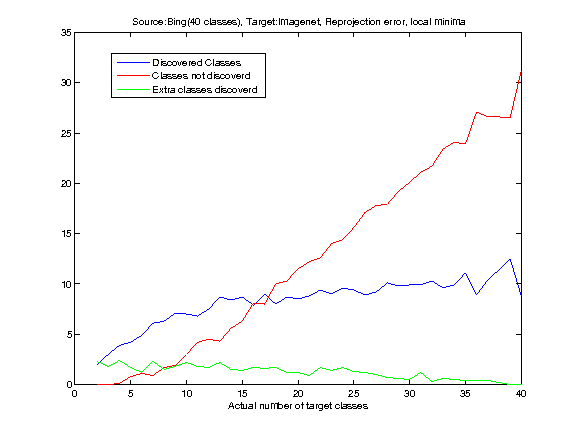}\label{fig:e2f1}} \hfill
\subfloat[Using Subspace Alignment Error and First Local Minimum]{\includegraphics[width=0.47\textwidth]{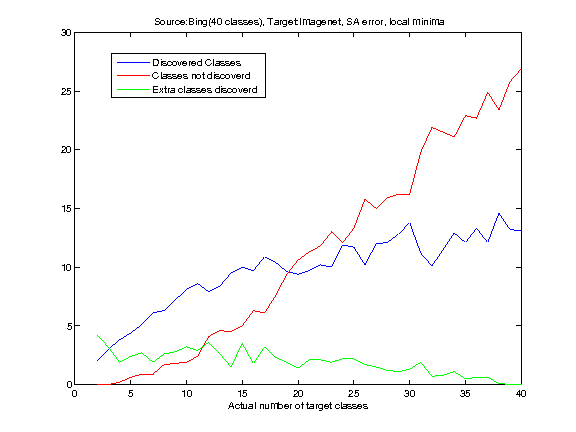}\label{fig:e2f3}}\\
\subfloat[Using Reprojection Error and Global Minimum]{\includegraphics[width=0.47\textwidth]{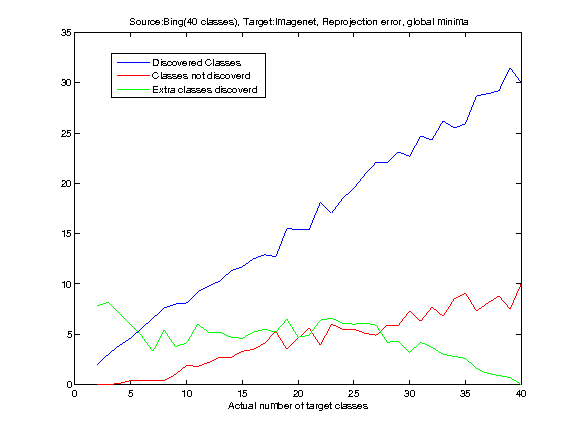}\label{fig:e2f2}}\hfill
\subfloat[Using Subspace Alignment Error and Global Minimum]{\includegraphics[width=0.47\textwidth]{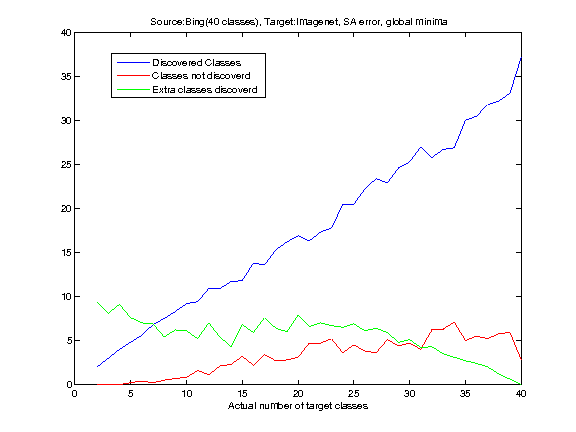}\label{fig:e2f4}}
\caption{Performance of the Evolution Step for different sizes of the target label set (x-axis). Source: Bing, Target: Imagenet. Blue: Number of target categories covered in the final selected set $C_{train}$. Red: Number of target categories missed in the final set. Green: Number of categories not present in the target but selected in the final set.}\label{fig:e2}
\end{figure}
\begin{figure}[H]
  \centering
\subfloat[Using Reprojection Error and  First Local Minimum]{\includegraphics[width=0.47\textwidth]{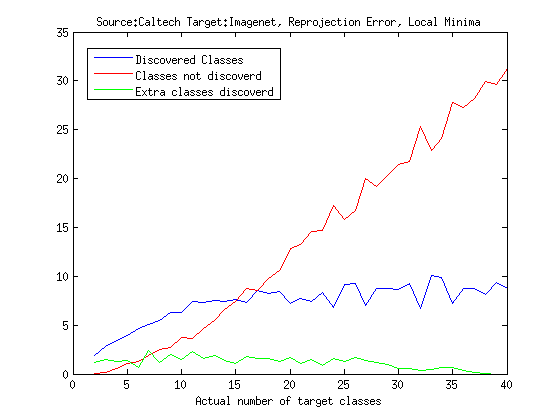}\label{fig:e3f1}} \hfill
\subfloat[Using Subspace Alignment Error and First Local Minimum]{\includegraphics[width=0.47\textwidth]{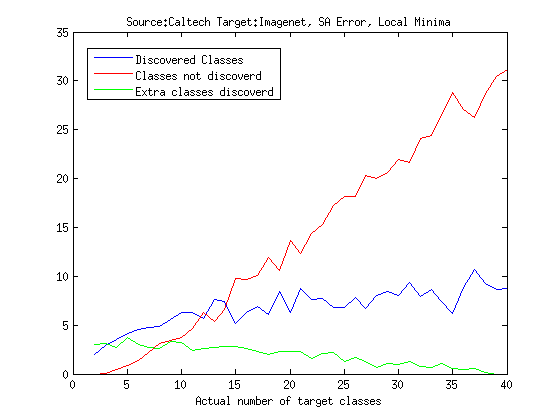}\label{fig:e3f3}}\\
\subfloat[Using Reprojection Error and Global Minimum]{\includegraphics[width=0.47\textwidth]{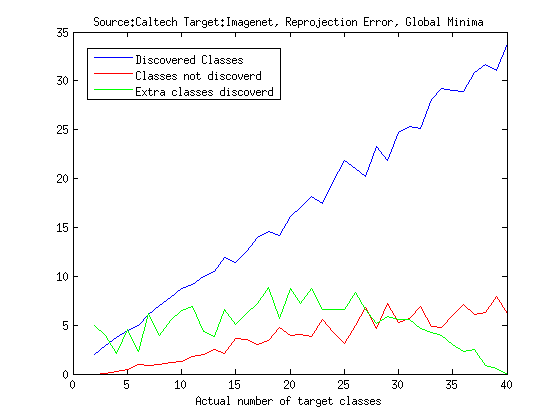}\label{fig:e3f2}}\hfill
\subfloat[Using Subspace Alignment Error and Global Minimum]{\includegraphics[width=0.47\textwidth]{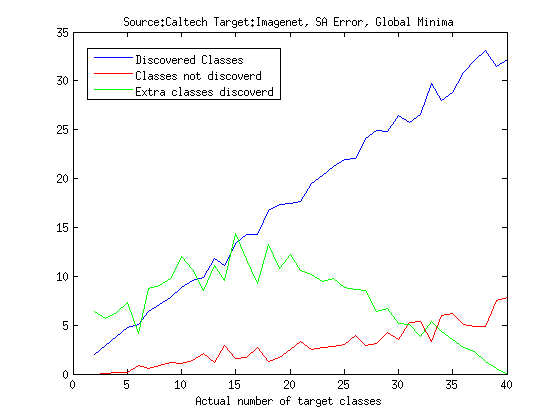}\label{fig:e3f4}}
\caption{Performance of the Evolution Step for different sizes of the target label set (x-axis). Source: Caltech, Target: Imagenet. Blue: Number of target categories covered in the final selected set $C_{train}$. Red: Number of target categories missed in the final set. Green: Number of categories not present in the target but selected in the final set.}\label{fig:e3}
\end{figure}
\begin{figure}[H]
  \centering
\subfloat[Using Reprojection Error and  First Local Minimum]{\includegraphics[width=0.47\textwidth]{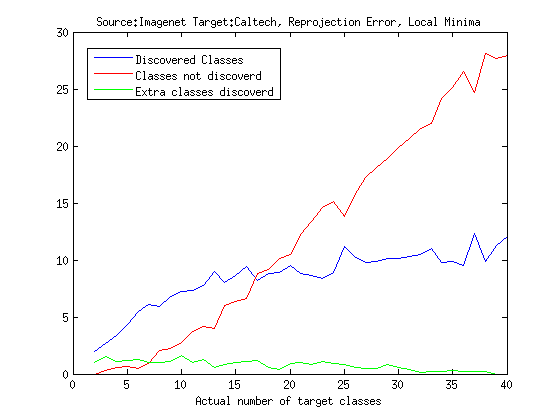}\label{fig:e4f1}} \hfill
\subfloat[Using Subspace Alignment Error and First Local Minimum]{\includegraphics[width=0.47\textwidth]{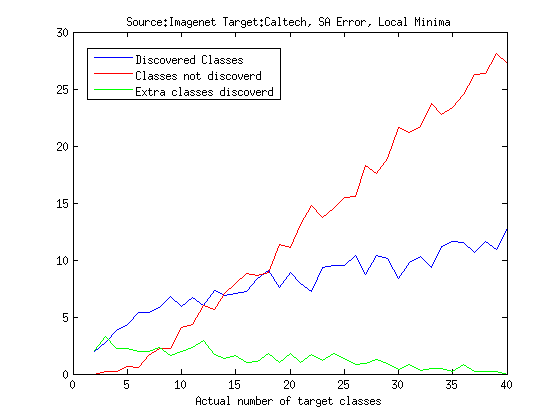}\label{fig:e4f3}}\\
\subfloat[Using Reprojection Error and Global Minimum]{\includegraphics[width=0.47\textwidth]{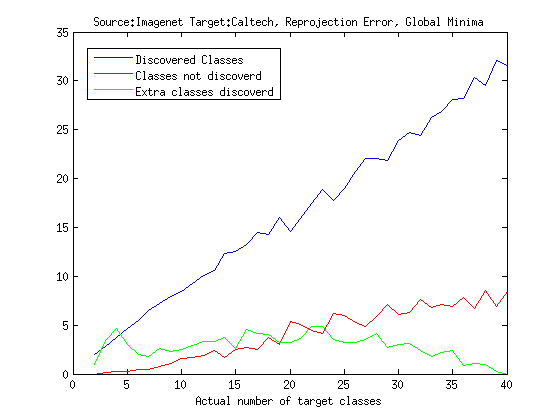}\label{fig:e4f2}}\hfill
\subfloat[Using Subspace Alignment Error and Global Minimum]{\includegraphics[width=0.47\textwidth]{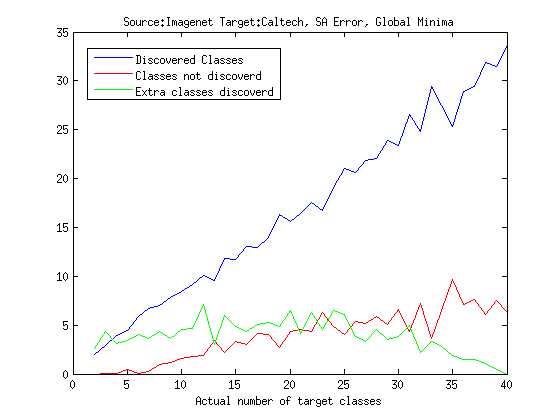}\label{fig:e4f4}}
  \caption{Performance of the Evolution Step for different sizes of the target label set (x-axis). Source: Imagenet, Target: Caltech. Blue: Number of target categories covered in the final selected set $C_{train}$. Red: Number of target categories missed in the final set. Green: Number of categories not present in the target but selected in the final set.}\label{fig:e4}
\end{figure}

\section{Baseline accuracy table}

Section 6.4 of the paper gives benchmark results for our algorithm with Subspace Alignment as adaptation technique. In table \ref{table:sa} we list the same result with large sizes for the target label set.

\begin{table}[H]
\begin{center}
\begin{adjustbox}{width=1\textwidth}
\begin{tabular}{|c|c|c|c|}
\hline
Number of Target & Source Categories = Target  & Available Source  & Predicted Target  \\ 
Categories & Categories (Oracle) & Categories & Categories(Our algorithm) \\
\hline
2 & 93.4726 & 66.3185 & \textbf{92.6893}\\
\hline
3 & 81.0219 & 46.5328 & \textbf{71.7153}\\
\hline
4 & 88.9764 & \textbf{70.0787} & 64.5669\\
\hline
5 & 87.9594 & 70.0887 & \textbf{74.1445}\\
\hline
6 & 86.7978 & 69.3820 & \textbf{72.2846}\\
\hline
7 & 88.9982 & 79.7787 & \textbf{82.9133}\\
\hline
8 & 80.2390 & 67.7291 & \textbf{69.8008}\\
\hline
9 & 80.7256 & 65.4573 & \textbf{66.1376}\\
\hline
10 & 83.4081 & 70.5834 & \textbf{76.0060}\\
\hline
13 & 73.6016 & 60.8458 & \textbf{70.1910}\\
\hline
16 & 76.3562 & 53.9918 & \textbf{63.7155}\\
\hline
19 & 65.8081 & 62.5607 & \textbf{65.1362}\\
\hline
21 & 76.2362 & 67.3071 & \textbf{68.6917}\\
\hline
24 & 71.8616 & 64.0857 & \textbf{67.8913}\\
\hline
27 & 67.2504 & 61.5368 & \textbf{63.5464}\\
\hline
30 & 66.7140 & 60.5018 & \textbf{61.8877}\\
\hline
\end{tabular}
\end{adjustbox}
\vspace{0.2cm}
\caption{Performance of our algorithm with Subspace Alignment as adaptation technique. Source Dataset: Bing,  Target Dataset:Caltech}
\label{table:sa}
\end{center}
\end{table}
\section{Visual Example for Multi-Source domain adaptation}

As shown in the paper our algorithm performs very well when working with multiple source domains. We give an illustrative example using the bottle category of Amazon, Webcam and DSLR domains.
Figure \ref{fig:bottles} shows some example images from these three domains. It can be clearly seen that DSLR and Webcam have very similar images for the bottle category whereas images in Amazon are very different from those in DSLR and Webcam. If we consider DSLR as target dataset then we expect the projection error for Webcam as source to be smaller than that for Amazon as source. Table \ref{table:bottles} confirms this intuition for both Subspace Alignment error and Reprojection error.

\begin{figure}[H]
\centering
\includegraphics[width=0.9\textwidth]{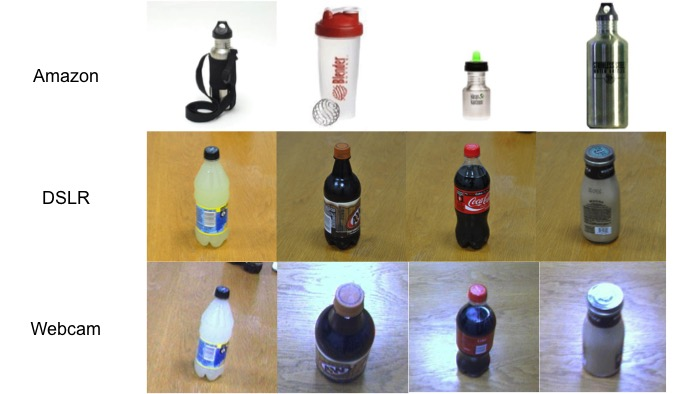}
\caption{Bottle Category: Amazon vs DSLR vs Webcam}
\label{fig:bottles}
\end{figure}

\begin{table}[H]
\centering
\begin{tabular}{|c|c|c|}
\hline
Source & Reprojection Error & Subspace Alignment Error \\
\hline
Amazon & 863.1376 & 2.8387\\
\hline
Webcam & \textbf{388.1430} & \textbf{2.5587}\\
\hline
\end{tabular}
\caption{Projection Errors on Bottle category, Target: DSLR}
\label{table:bottles}
\end{table}
